# Supplementary material for: Grounded Conversation Generation as Guided Traverses in Commonsense Knowledge Graphs
Source: arXiv:1911.02707 source file (2020-05-05)
Supplement: Supplementary file 1 [file appendix_ablation_novelty.tex]

\begin{table*}[h]
\centering
\small
\begin{tabular}{l|c|c|c|c|c|c}
\hline \hline
Version     & Rouge-1 & Rouge-2 & Rouge-L & Meteor & Dist-1 & Dist-2  \\ \hline
Base & 0.1526 & 0.0192 & 0.1242 & 0.0665 & 0.0129 & 0.0542 \\ \hline
Rand & 0.1537 & 0.0193 & 0.1244 & 0.0657 & 0.0134 & 0.0567 \\ \hline
Distract & 0.1562 & 0.0201 & 0.1256 & 0.0641 & 0.0153 & 0.0699 \\ \hline
Full      & \textbf{0.2101} & \textbf{0.0395} & \textbf{0.1719} & \textbf{0.0874} & \textbf{0.0203} & \textbf{0.1126} \\ \hline \hline
\end{tabular}
\caption{\label{tab: appendix ablation diversity}Rouge and Meteor for Relevance and Dist for Diversity of Ablation Study. Rouge and Meteor are calculated to evaluate the relevance between generated responses and golden responses. The Dist indicates the diversity of generated responses.}
\end{table*}
