# Supplementary material for: Grounded Conversation Generation as Guided Traverses in Commonsense Knowledge Graphs
Source: arXiv:1911.02707 source file (2020-05-05)
Supplement: Supplementary file 3 [file final_appendix_parameters.tex]

\begin{table}[t]
\centering
\small
\begin{tabular}{c|c}
\hline  \hline
Model     & Number of Parameters \\ \hline
GPT-2 (conv)   & 124M      \\ \hline
ConceptFlow    & 35M   \\ \hline \hline

\end{tabular}
\caption{\label{tab: parameters}Statistics of Model Parameters.}
\end{table}
