# Supplementary material for: Grounded Conversation Generation as Guided Traverses in Commonsense Knowledge Graphs
Source: arXiv:1911.02707 source file (2020-05-05)
Supplement: Supplementary file 4 [file final_appendix_tophuman.tex]

\begin{table}[t]
\centering
\small
\begin{tabular}{c|c|c}
\hline  \hline
Model     & Appropriateness & Informativeness \\ \hline
CCM   & 0.73 & 0.66 \\ \hline
GPT-2 (conv)  & 1.18  & 1.07 \\ \hline 
ConceptFlow & 1.74 & 1.62  \\ \hline \hline
\end{tabular}
\caption{\label{tab: top response}The average number of times being the top response for each case in human evaluation.}
\end{table}
